# Supplementary material for: The complete NLO corrections to dijet hadroproduction
Source: arXiv:1612.06548 ancillary file (2017-04-07)
Supplement: Supplementary file 1 [file xsec_table.pdf]

## Additional validation material for publication

*”The complete NLO corrections to dijet hadroproduction”*

*R.Frederix, S.Frixione, V.Hirschi, D.Pagani, H.-S. Shao. M.Zaro*

This auxiliary material includes two tables presenting semi-inclusive cross-sections of dijet production at LHC 13 TeV for slices of phase-space defined within successive values of partonic  $H_T$ , defined as the sum of the transverse momenta of all final state partons, that is:

$$H_T = \sum_{i=1, n_{\text{partons}}} \sqrt{p_{x,i}^2 + p_{y,i}^2}.$$

Even though partonic  $H_T$  is an unphysical quantity, it has the advantage of being correlated to the physical *jet*  $H_T$  while remaining independent of any jet algorithm. This dataset is therefore well suited for reproducibility purposes and can be used as a benchmark for alternative implementations.

These results within different kinematic regimes and for semi-inclusive cross-sections of individual orders  $\mathcal{O}(\alpha_s^m \alpha^n |_{m+n=2,3})$  allow sensitivity to various sub-leading contributions which would otherwise be well below Monte-Carlo accuracy in more inclusive quantities.

We refer the reader to sect. 4 of the publication aforementioned for the model parameters, simulation setup and *dijet* acceptance cuts (eqs. 4.1 and 4.10), and to sect. 3 for the photon jet definition. Regarding the contribution labeled  $\mathcal{O}(\alpha_s^2 \alpha)$ ,  $1\gamma$ -tagged, it is important to stress that we consider here the quantity subtracted from *dijet correlation* observables and as such it only includes configurations where the tagged photon belongs to either of the two hardest jets.

Hard scale uncertainties on pure next-to-leading order contributions are not reported since they are not meaningful when taken separately from their leading order counterpart.

The integration of all contributions factorizing different coupling order combinations was performed in a single run, using a fixed number of iterations and phase-space points so as to retain sensitivity to sub-leading contributions. We note however that integrating such contributions separately would improve numerical stability.

| Contribution [pb] |                                                      | 120 GeV < $H_T$ < 240 GeV      |                |       | 240 GeV < $H_T$ < 480 GeV       |                |       | 480 GeV < $H_T$ < 960 GeV       |                |       |
|-------------------|------------------------------------------------------|--------------------------------|----------------|-------|---------------------------------|----------------|-------|---------------------------------|----------------|-------|
| all orders        |                                                      | 2.509 ±0.005 ·10 <sup>6</sup>  | +8.7%<br>-9.7% | ±1%   | 1.066 ±0.001 ·10 <sup>6</sup>   | +22%<br>-16%   | ±0.9% | 4.887 ±0.004 ·10 <sup>4</sup>   | +21%<br>-17%   | ±1.3% |
| LO                | $\mathcal{O}(\alpha_s^2)$                            | 1.864 ±0.001 ·10 <sup>6</sup>  | +26%<br>-20%   | ±0.9% | 4.361 ±0.002 ·10 <sup>5</sup>   | +25%<br>-19%   | ±0.9% | 2.1242 ±0.0006 ·10 <sup>4</sup> | +28%<br>-21%   | ±1.3% |
|                   | $\mathcal{O}(\alpha_s\alpha)$                        | 1.711 ±0.001 ·10 <sup>3</sup>  | +19%<br>-16%   | ±3.4% | 6.824 ±0.004 ·10 <sup>2</sup>   | +13%<br>-11%   | ±3.9% | 7.810 ±0.003 ·10 <sup>1</sup>   | +11%<br>-9.4%  | ±3.6% |
|                   | $\mathcal{O}(\alpha_s\alpha)$ , no $\gamma$ -PDF     | 1.595 ±0.001 ·10 <sup>3</sup>  | +18%<br>-16%   | ±1%   | 6.388 ±0.005 ·10 <sup>2</sup>   | +13%<br>-11%   | ±1.3% | 7.391 ±0.005 ·10 <sup>1</sup>   | +12%<br>-9.8%  | ±1.4% |
|                   | $\mathcal{O}(\alpha_s\alpha)$ , 1 $\gamma$ -tagged   | 8.104 ±0.003 ·10 <sup>2</sup>  | +17%<br>-15%   | ±1%   | 2.4973 ±0.0007 ·10 <sup>2</sup> | +11%<br>-10%   | ±0.8% | 1.8442 ±0.0003 ·10 <sup>1</sup> | +14%<br>-12%   | ±0.5% |
|                   | $\mathcal{O}(\alpha_s\alpha^2)$                      | 8.154 ±0.004 ·10 <sup>2</sup>  | +6.2%<br>-7.5% | ±1.1% | 4.380 ±0.002 ·10 <sup>2</sup>   | +2.1%<br>-3%   | ±1%   | 5.550 ±0.001 ·10 <sup>1</sup>   | +2.3%<br>-2.5% | ±1%   |
|                   | $\mathcal{O}(\alpha^2)$ , no $\gamma$ -PDF           | 8.152 ±0.004 ·10 <sup>2</sup>  | +6.2%<br>-7.5% | ±1.1% | 4.379 ±0.002 ·10 <sup>2</sup>   | +2.1%<br>-3%   | ±1%   | 5.545 ±0.002 ·10 <sup>1</sup>   | +2.3%<br>-2.5% | ±1%   |
|                   | $\mathcal{O}(\alpha^2)$ , 2 $\gamma$ -tagged         | 7.227 ±0.008 ·10 <sup>-1</sup> | +6.6%<br>-7.9% | ±1.6% | 2.818 ±0.002 ·10 <sup>-1</sup>  | +2.7%<br>-3.7% | ±1.8% | 2.934 ±0.001 ·10 <sup>-2</sup>  | +1.6%<br>-1.9% | ±1.7% |
| NLO               | $\mathcal{O}(\alpha_s^3)$                            | 6.45 ±0.04 ·10 <sup>5</sup>    |                | ±1.3% | 6.26 ±0.01 ·10 <sup>5</sup>     |                | ±0.9% | 2.756 ±0.003 ·10 <sup>4</sup>   |                | ±1.3% |
|                   | $\mathcal{O}(\alpha_s^2\alpha)$                      | -2.93 ±0.03 ·10 <sup>3</sup>   |                | ±0.9% | -7.59 ±0.04 ·10 <sup>2</sup>    |                | ±4%   | -1.556 ±0.003 ·10 <sup>2</sup>  |                | ±2%   |
|                   | $\mathcal{O}(\alpha_s^2\alpha)$ , no $\gamma$ -PDF   | -2.92 ±0.03 ·10 <sup>3</sup>   |                | ±0.9% | -8.07 ±0.04 ·10 <sup>2</sup>    |                | ±0.9% | -1.596 ±0.003 ·10 <sup>2</sup>  |                | ±0.6% |
|                   | $\mathcal{O}(\alpha_s^2\alpha)$ , 1 $\gamma$ -tagged | 4.51 ±0.04 ·10 <sup>2</sup>    |                | ±0.9% | 4.012 ±0.008 ·10 <sup>2</sup>   |                | ±0.6% | 2.690 ±0.004 ·10 <sup>1</sup>   |                | ±0.5% |
|                   | $\mathcal{O}(\alpha_s\alpha^2)$                      | 1.585 ±0.004 ·10 <sup>3</sup>  |                | ±1%   | 1.014 ±0.002 ·10 <sup>3</sup>   |                | ±0.7% | 8.31 ±0.01 ·10 <sup>1</sup>     |                | ±0.5% |
|                   | $\mathcal{O}(\alpha_s\alpha^2)$ , no $\gamma$ -PDF   | 1.571 ±0.004 ·10 <sup>3</sup>  |                | ±0.9% | 1.007 ±0.002 ·10 <sup>3</sup>   |                | ±0.7% | 8.37 ±0.04 ·10 <sup>1</sup>     |                | ±0.5% |
|                   | $\mathcal{O}(\alpha_s\alpha^2)$ , 2 $\gamma$ -tagged | 2.8 ±0.2 ·10 <sup>-1</sup>     |                | ±1.3% | 7.42 ±0.03 ·10 <sup>-1</sup>    |                | ±0.8% | 1.044 ±0.002 ·10 <sup>-1</sup>  |                | ±0.7% |
|                   | $\mathcal{O}(\alpha^3)$                              | 7.39 ±0.07                     |                | ±40%  | 3.82 ±0.04                      |                | ±110% | -1.877 ±0.007                   |                | ±29%  |
|                   | $\mathcal{O}(\alpha^3)$ , no $\gamma$ -PDF           | -3.9 ±0.6 ·10 <sup>-1</sup>    |                | ±16%  | -3.47 ±0.03                     |                | ±1.6% | -3.021 ±0.007                   |                | ±1.1% |

Table 1: Semi-inclusive cross-sections for phase-space slices of partonic  $H_T$  (scalar sum of the transverse momenta of all final state partons) from 120 GeV to 960 GeV. In order, results are given as the semi-inclusive cross-section, the numerical integration error, the hard scale uncertainty (for LO and all orders results only) and PDF uncertainty. See main text for simulation parameters, in particular the jet definition and cuts, as well as for the tagged photon jet definition.

| Contribution [pb] |                                                      | 960 GeV < $H_T$ < 2 TeV |              |                 |                                                          | 2 TeV < $H_T$ < 4 TeV |        |              |                 | 4 TeV < $H_T$ < $\infty$                                |             |        |              |                 |                                                        |             |
|-------------------|------------------------------------------------------|-------------------------|--------------|-----------------|----------------------------------------------------------|-----------------------|--------|--------------|-----------------|---------------------------------------------------------|-------------|--------|--------------|-----------------|--------------------------------------------------------|-------------|
| all orders        |                                                      | 1.398                   | $\pm 0.001$  | $\cdot 10^3$    | $\begin{smallmatrix} +20\% \\ -16\% \end{smallmatrix}$   | $\pm 2.1\%$           | 1.623  | $\pm 0.001$  | $\cdot 10^1$    | $\begin{smallmatrix} +18\% \\ -16\% \end{smallmatrix}$  | $\pm 3.3\%$ | 6.512  | $\pm 0.003$  | $\cdot 10^{-2}$ | $\begin{smallmatrix} +17\% \\ -15\% \end{smallmatrix}$ | $\pm 5.4\%$ |
| LO                | $\mathcal{O}(\alpha_s^2)$                            | 6.550                   | $\pm 0.001$  | $\cdot 10^2$    | $\begin{smallmatrix} +31\% \\ -22\% \end{smallmatrix}$   | $\pm 2.1\%$           | 7.980  | $\pm 0.002$  |                 | $\begin{smallmatrix} +33\% \\ -23\% \end{smallmatrix}$  | $\pm 3.2\%$ | 3.1737 | $\pm 0.0006$ | $\cdot 10^{-2}$ | $\begin{smallmatrix} +35\% \\ -25\% \end{smallmatrix}$ | $\pm 5.6\%$ |
|                   | $\mathcal{O}(\alpha_s \alpha)$                       | 7.122                   | $\pm 0.002$  |                 | $\begin{smallmatrix} +14\% \\ -12\% \end{smallmatrix}$   | $\pm 3.3\%$           | 3.290  | $\pm 0.001$  | $\cdot 10^{-1}$ | $\begin{smallmatrix} +18\% \\ -14\% \end{smallmatrix}$  | $\pm 3.8\%$ | 4.3355 | $\pm 0.0009$ | $\cdot 10^{-3}$ | $\begin{smallmatrix} +23\% \\ -18\% \end{smallmatrix}$ | $\pm 6.8\%$ |
|                   | $\mathcal{O}(\alpha_s \alpha)$ , no $\gamma$ -PDF    | 6.822                   | $\pm 0.002$  |                 | $\begin{smallmatrix} +15\% \\ -12\% \end{smallmatrix}$   | $\pm 1.8\%$           | 3.220  | $\pm 0.001$  | $\cdot 10^{-1}$ | $\begin{smallmatrix} +18\% \\ -14\% \end{smallmatrix}$  | $\pm 3.2\%$ | 4.137  | $\pm 0.002$  | $\cdot 10^{-3}$ | $\begin{smallmatrix} +24\% \\ -18\% \end{smallmatrix}$ | $\pm 3.7\%$ |
|                   | $\mathcal{O}(\alpha_s \alpha)$ , $1\gamma$ -tagged   | 8.371                   | $\pm 0.002$  | $\cdot 10^{-1}$ | $\begin{smallmatrix} +18\% \\ -15\% \end{smallmatrix}$   | $\pm 0.9\%$           | 1.3700 | $\pm 0.0004$ | $\cdot 10^{-2}$ | $\begin{smallmatrix} +23\% \\ -18\% \end{smallmatrix}$  | $\pm 2.6\%$ | 5.090  | $\pm 0.001$  | $\cdot 10^{-5}$ | $\begin{smallmatrix} +29\% \\ -21\% \end{smallmatrix}$ | $\pm 10\%$  |
|                   | $\mathcal{O}(\alpha_s \alpha^2)$                     | 3.828                   | $\pm 0.001$  |                 | $\begin{smallmatrix} +6.7\% \\ -6\% \end{smallmatrix}$   | $\pm 1\%$             | 1.1066 | $\pm 0.0007$ | $\cdot 10^{-1}$ | $\begin{smallmatrix} +11\% \\ -9.2\% \end{smallmatrix}$ | $\pm 1.6\%$ | 9.778  | $\pm 0.004$  | $\cdot 10^{-4}$ | $\begin{smallmatrix} +16\% \\ -13\% \end{smallmatrix}$ | $\pm 4.8\%$ |
|                   | $\mathcal{O}(\alpha_s \alpha^2)$ , no $\gamma$ -PDF  | 3.824                   | $\pm 0.002$  |                 | $\begin{smallmatrix} +6.7\% \\ -6.1\% \end{smallmatrix}$ | $\pm 1.1\%$           | 1.1048 | $\pm 0.0007$ | $\cdot 10^{-1}$ | $\begin{smallmatrix} +11\% \\ -9.2\% \end{smallmatrix}$ | $\pm 2\%$   | 9.718  | $\pm 0.009$  | $\cdot 10^{-4}$ | $\begin{smallmatrix} +16\% \\ -13\% \end{smallmatrix}$ | $\pm 3.9\%$ |
|                   | $\mathcal{O}(\alpha_s \alpha^2)$ , $2\gamma$ -tagged | 1.8351                  | $\pm 0.0008$ | $\cdot 10^{-3}$ | $\begin{smallmatrix} +6.2\% \\ -5.7\% \end{smallmatrix}$ | $\pm 2.3\%$           | 4.029  | $\pm 0.003$  | $\cdot 10^{-5}$ | $\begin{smallmatrix} +11\% \\ -9.4\% \end{smallmatrix}$ | $\pm 4.9\%$ | 1.8507 | $\pm 0.0008$ | $\cdot 10^{-7}$ | $\begin{smallmatrix} +17\% \\ -14\% \end{smallmatrix}$ | $\pm 23\%$  |
| NLO               | $\mathcal{O}(\alpha_s^3)$                            | 7.401                   | $\pm 0.007$  | $\cdot 10^2$    |                                                          | $\pm 2.2\%$           | 8.134  | $\pm 0.008$  |                 |                                                         | $\pm 3.4\%$ | 3.035  | $\pm 0.002$  | $\cdot 10^{-2}$ |                                                        | $\pm 5.9\%$ |
|                   | $\mathcal{O}(\alpha_s^2 \alpha)$                     | -1.277                  | $\pm 0.002$  | $\cdot 10^1$    |                                                          | $\pm 1.8\%$           | -3.17  | $\pm 0.01$   | $\cdot 10^{-1}$ |                                                         | $\pm 3.8\%$ | -1.495 | $\pm 0.007$  | $\cdot 10^{-3}$ |                                                        | $\pm 12\%$  |
|                   | $\mathcal{O}(\alpha_s^2 \alpha)$ , no $\gamma$ -PDF  | -1.298                  | $\pm 0.002$  | $\cdot 10^1$    |                                                          | $\pm 1.1\%$           | -3.17  | $\pm 0.02$   | $\cdot 10^{-1}$ |                                                         | $\pm 3.1\%$ | -1.594 | $\pm 0.006$  | $\cdot 10^{-3}$ |                                                        | $\pm 9\%$   |
|                   | $\mathcal{O}(\alpha_s^2 \alpha)$ , $1\gamma$ -tagged | 1.084                   | $\pm 0.002$  |                 |                                                          | $\pm 0.9\%$           | 1.759  | $\pm 0.003$  | $\cdot 10^{-2}$ |                                                         | $\pm 2.1\%$ | 8.018  | $\pm 0.009$  | $\cdot 10^{-5}$ |                                                        | $\pm 5.3\%$ |
|                   | $\mathcal{O}(\alpha_s \alpha^2)$                     | 3.59                    | $\pm 0.01$   |                 |                                                          | $\pm 1\%$             | 2.48   | $\pm 0.05$   | $\cdot 10^{-2}$ |                                                         | $\pm 8.5\%$ | -5.67  | $\pm 0.03$   | $\cdot 10^{-4}$ |                                                        | $\pm 10\%$  |
|                   | $\mathcal{O}(\alpha_s \alpha^2)$ , no $\gamma$ -PDF  | 3.56                    | $\pm 0.01$   |                 |                                                          | $\pm 1.1\%$           | 2.69   | $\pm 0.07$   | $\cdot 10^{-2}$ |                                                         | $\pm 7.1\%$ | -5.57  | $\pm 0.06$   | $\cdot 10^{-4}$ |                                                        | $\pm 8.5\%$ |
|                   | $\mathcal{O}(\alpha_s \alpha^2)$ , $2\gamma$ -tagged | 7.00                    | $\pm 0.01$   | $\cdot 10^{-3}$ |                                                          | $\pm 1.1\%$           | 1.553  | $\pm 0.003$  | $\cdot 10^{-4}$ |                                                         | $\pm 2.9\%$ | 6.957  | $\pm 0.006$  | $\cdot 10^{-7}$ |                                                        | $\pm 12\%$  |
|                   | $\mathcal{O}(\alpha^3)$                              | -3.95                   | $\pm 0.01$   | $\cdot 10^{-1}$ |                                                          | $\pm 16\%$            | -2.05  | $\pm 0.01$   | $\cdot 10^{-2}$ |                                                         | $\pm 18\%$  | -2.34  | $\pm 0.01$   | $\cdot 10^{-4}$ |                                                        | $\pm 30\%$  |
|                   | $\mathcal{O}(\alpha^3)$ , no $\gamma$ -PDF           | -5.050                  | $\pm 0.006$  | $\cdot 10^{-1}$ |                                                          | $\pm 1.3\%$           | -2.31  | $\pm 0.01$   | $\cdot 10^{-2}$ |                                                         | $\pm 9.7\%$ | -3.001 | $\pm 0.004$  | $\cdot 10^{-4}$ |                                                        | $\pm 4.4\%$ |

Table 2: Semi-inclusive cross-sections for phase-space slices of partonic  $H_T$  (scalar sum of the transverse momenta of all final state partons) from 120 GeV to 960 GeV. In order, results are given as the semi-inclusive cross-section, the numerical integration error, the hard scale uncertainty (for LO and all orders results only) and PDF uncertainty. See main text for simulation parameters, in particular the jet definition and cuts, as well as for the tagged photon jet definition.
